# Supplementary material for: Material Decomposition in Photon-Counting Computed Tomography with Diffusion Models: Comparative Study and Hybridization with Variational Regularizers
Source: arXiv:2503.15383 source file (2026-01-13)
Supplement: Supplementary file 1 [file appendix.tex]

\section*{Appendix}

Figure~\ref{fig:ResultatsLowCount_annex} and Figure~\ref{fig:ResultatsSparseView_annex} show the relative error map and profile lines of the reconstructed images from Experiment 1. The noise present in \ac{FBP} and \ac{LBFGS} is clearly visible on the profile lines. The observable oversmoothing of U-Net-I in Figure \ref{fig:ResultatsSparseView} is also visible in the profile line of the sparse-view data experiment.

\input{figures/Resultats_annexe_Lowcount}
\vspace{2cm}
\input{figures/Resultats_annexe_Sparseview}
